# Supplementary material for: EnigmaToM: Improve LLMs' Theory-of-Mind Reasoning Capabilities with Neural Knowledge Base of Entity States
Source: arXiv:2503.03340 source file (2025-06-02)
Supplement: Supplementary file 1 [file annotation_guideline.pdf]

# Annotation Guideline for Evaluation of Neural Knowledge Base

---

## Task Formulation

In this task, you will be responsible for evaluating the quality of entity state information generated by two Neural Knowledge Base. You will be given a set of **Questions** in the `question` column, an **event** or **utterance** in the `event` column and a **entity state information** generated from a neural knowledge bank in the `xxx_states` column.

You will be annotating the following two aspects of the generated entity state information:

1. **Relavance**: whether the generated entity state knowledge is helpful with answering the questions.
2. **Accuracy**: whether the entity state can be entailed from the given event/utterance.

For both tasks, choose `yes` if you believe that the entity state is relevant/accurate and choose `No` otherwise.

Note that all of the entity state follows a semi-structured formulation:

- [Attribute] of [Entity] is [Current State]

In the `Relevance` annotation task, you only need to pay attention to the `[Attribute] of [Entity]`.

In the `Accuracy` annotation task, you need to consider the complete entity state description.

## Examples

| QUESTION                                                         | EVENT                                     | STATE                                          |
|------------------------------------------------------------------|-------------------------------------------|------------------------------------------------|
| Where does Abigail think that Benjamin searches for the pumpkin? | Abigail moved the pumpkin to the bathtub. | - <b>location of the pumpkin is in bathtub</b> |

In this example, we see that the `Location of the Pumpkin` is important in answering the question. **Therefore, we mark the relevance as `yes`.**

We see that there exists an entailment relationship between `Event` and `State`. **Therefore, we mark the accuracy as `yes`**

| QUESTION                                                         | EVENT                       | STATE                                     |
|------------------------------------------------------------------|-----------------------------|-------------------------------------------|
| Where does Abigail think that Benjamin searches for the pumpkin? | Chloe entered the workshop. | - <b>location of Chloe is in workshop</b> |

In this example, we see that the `Location of the Chloe` is not related to the question. **Therefore, we mark the relevance as `No`.**

We see that there exists an entailment relationship between `Event` and `State`. **Therefore, we mark the accuracy as `Yes`**

| QUESTION                                                         | EVENT                                     | STATE                                      |
|------------------------------------------------------------------|-------------------------------------------|--------------------------------------------|
| Where does Abigail think that Benjamin searches for the pumpkin? | Abigail moved the pumpkin to the bathtub. | - <b>location of Abigail is in bathtub</b> |

In this example, we see that the `Location of the Abigail` is important in answering the question. **Therefore, we mark the relevance as `yes`.**

However, it is unlikely that Abigail needs to enter the bathtub to place the pumpkin. **Therefore, there does not exist an entailment relationship between `Event` and `state`. Therefore, we mark the accuracy as `No`.**

| QUESTION                                                         | EVENT                       | STATE                                    |
|------------------------------------------------------------------|-----------------------------|------------------------------------------|
| Where does Abigail think that Benjamin searches for the pumpkin? | Chloe entered the workshop. | - <b>location of Chloe is in kitchen</b> |

In this example, we see that the `Location of the Chloe` is not related to the question. **Therefore, we mark the relevance as `No`.**

We see that there does not exist an entailment relationship between `Event` and `State`. **Therefore, we mark the accuracy as `No`**
